# Supplementary material for: Bayesian Deep Learning Via Expectation Maximization and Turbo Deep Approximate Message Passing
Source: arXiv:2402.07366 source file (2024-06-09)
Supplement: Supplementary file 1 [file supplementarymaterial_revised_0331.pdf]

# SUPPLEMENTARY MATERIAL FOR

Bayesian Federated Learning Via Expectation-Maximization and Turbo Deep Approximate Message Passing

Wei Xu, An Liu, Yiting Zhang and Vincent Lau

## S-I. DERIVATION OF APPROXIMATE MESSAGE PASSING WITHIN LAYER $l$

The joint PDF of $\boldsymbol{u}_{l-1}^{r_k}, \boldsymbol{\theta}_l, \boldsymbol{z}_l^{r_k}$ associated with $\mathcal{G}_{r_k}$ is

$$\begin{aligned} p\left(\boldsymbol{u}_{l-1}^{r_k}, \boldsymbol{\theta}_l, \boldsymbol{z}_l^{r_k}\right) \propto & \exp\left(\sum_{n=1}^{N_{l-1}} \sum_{i \in \mathcal{I}_{r_k}} \triangle_{h_{l-1,ni} \rightarrow u_{l-1,ni}}\right) \\ & \times \exp\left(\sum_{m=1}^{N_l} \sum_{n=1}^{N_{l-1}} \triangle_{h_{l,mn}^W \rightarrow W_{l,mn}} + \sum_{m=1}^{N_l} \triangle_{h_{l,m}^b \rightarrow b_{l,m}}\right) \\ & \times \prod_{m=1}^{N_l} \prod_{i \in \mathcal{I}_{r_k}} \delta\left(z_{l,mi} - \left(\sum_{n=1}^{N_{l-1}} W_{l,mn} u_{l-1,ni} + b_{l,m}\right)\right) \\ & \times \exp\left(\sum_{m=1}^{N_l} \sum_{i \in \mathcal{I}_{r_k}} \triangle_{z_{l,mi} \rightarrow f_{l,mi}}\right). \end{aligned}$$

The detailed factor graph is shown in Fig. 1. Here we denote by $\triangle_{a \rightarrow b}(t)$ the message from node $a$ to $b$ in iteration $t$, and by $\triangle_c(t)$ the marginal posterior computed at variable node $c$ in iteration $t$. However, the complexity of directly calculating the messages on edge in Fig. 1 based on sum product rule is high. In this paper, we approximate the messages to achieve a good tradeoff between the complexity and performance. Messages within a layer has similar expression to those considered in [*S1*], and we shall follow the general idea of the BiG-AMP framework in [*S1*] to approximate the messages. Specifically, we approximate the exponential messages as normal distributions through second order Taylor series expansion. As such, we only need to calculate the expectation and variance associated with the messages. For convenience, we note the expectation and variance of $\exp\left(\triangle_{a \rightarrow b}(t)\right)$ and $\exp\left(\triangle_c(t)\right)$ as $\mu_{a \rightarrow b}(t), v_{a \rightarrow b}(t)$ and $\mu_c(t), v_c(t)$, respectively. Besides, we form a scaling table I for variables as $I_k, N_l, N_{l-1} \rightarrow \infty$, where $I_k, N_l, N_{l-1} \sim O(N)$, similar to that mentioned in [*S1*]. We will neglect terms that vanish related to others in large system limit based on Table I in later approximations.

### A. Approximated Factor-to-Variable Messages

Here we approximate $\triangle_{f_{l,mi} \rightarrow b_{l,m}}, \triangle_{f_{l,mi} \rightarrow W_{l,mn}}$ and $\triangle_{f_{l,mi} \rightarrow u_{l-1,ni}}$ as logarithm of Gaussian. Firstly, for large $N_l$, the central-limit-theorem motivates the treatment of $z_{l,mi}$ as Gaussian:

$$\begin{aligned} \triangle_{f_{l,mi} \rightarrow x}(t) \approx & \log \int_{z_{l,mi}} \exp\left(\triangle_{z_{l,mi} \rightarrow f_{l,mi}}\right) \\ & \times N\left(z_{l,mi}; \mu_{z_{l,mi}|x}(t), v_{z_{l,mi}|x}(t)\right), \quad \text{(S1)} \end{aligned}$$

where $x$ represents any element in $\{b_{l,m}, W_{l,mn}, u_{l-1,ni} | \forall n\}$. $\mu_{z_{l,mi}|x}(t)$ and $v_{z_{l,mi}|x}(t)$ represent the expectation and variance of $z_{l,mi}$ conditioned on $x$ in iteration $t$, respectively. After omitting $O\left(\frac{1}{N}\right)$ terms, $\mu_{z_{l,mi}|x}(t)$ and $v_{z_{l,mi}|x}(t)$ are approximated as follows:

$$\begin{aligned} \mu_{z_{l,mi}|x}(t) \approx & \mu_{f_{l,mi} \rightarrow z_{l,mi}}(t) \\ & + \begin{cases} b_{l,m} - \mu_{b_{l,m}}(t) & x = b_{l,m} \\ \left(W_{l,mn} - \mu_{W_{l,mn}}(t)\right) \mu_{u_{l-1,ni} \rightarrow f_{l,mi}}(t) & x = W_{l,mn} \\ \mu_{W_{l,mn}}(t)\left(u_{l-1,mi} - \mu_{u_{l-1,ni} \rightarrow f_{l,mi}}(t)\right) & x = u_{l-1,ni} \end{cases}, \end{aligned}$$

$$\begin{aligned} v_{z_{l,mi}|x}(t) \approx & v_{f_{l,mi} \rightarrow z_{l,mi}}(t) \\ & + \begin{cases} 0 & x = b_{l,m} \\ \left(W_{l,mn}^2 - \mu_{W_{l,mn}}^2(t)\right) v_{u_{l-1,ni} \rightarrow f_{l,mi}}(t) & x = W_{l,mn} \\ v_{W_{l,mn} \rightarrow f_{l,mi}}(t)\left(u_{l-1,ni}^2 - \mu_{u_{l-1,ni}}^2(t)\right) & x = u_{l-1,ni} \end{cases}, \end{aligned}$$

where we define:

$$\begin{aligned} \mu_{f_{l,mi} \rightarrow z_{l,mi}}(t) = & \sum_{n=1}^{N_{l-1}} \mu_{W_{l,mn} \rightarrow f_{l,mi}}(t) \mu_{u_{l-1,ni} \rightarrow f_{l,mi}}(t) \\ & + \mu_{b_{l,m} \rightarrow f_{l,mi}}(t), \quad \text{(S2)} \end{aligned}$$

$$\begin{aligned} v_{f_{l,mi} \rightarrow z_{l,mi}}(t) = & \sum_{n=1}^{N_{l-1}} \mu_{W_{l,mn} \rightarrow f_{l,mi}}^2(t) v_{u_{l-1,ni} \rightarrow f_{l,mi}}(t) \\ & + \sum_{n=1}^{N_{l-1}} v_{W_{l,mn} \rightarrow f_{l,mi}}(t) \mu_{u_{l-1,ni} \rightarrow f_{l,mi}}^2(t) \\ & + \sum_{n=1}^{N_{l-1}} v_{W_{l,mn} \rightarrow f_{l,mi}}(t) v_{u_{l-1,ni} \rightarrow f_{l,mi}}(t) \\ & + v_{b_{l,m} \rightarrow f_{l,mi}}(t). \quad \text{(S3)} \end{aligned}$$

By applying Taylor series expansion to $\triangle_{f_{l,mi} \rightarrow x}(t)$ in $x$ about the point $\mu_x(t)$ and omit $O\left(\frac{1}{N^{3/2}}\right)$, we obtain:

$$\triangle_{f_{l,mi} \rightarrow b_{l,m}}(t) \approx A_{b_{l,m}^i}(t) b_{l,m} - \frac{1}{2} B_{b_{l,m}^i}(t) b_{l,m}^2, \quad \text{(S4)}$$

$$\triangle_{f_{l,mi} \rightarrow W_{l,mn}}(t) \approx A_{W_{l,mn}^i}(t) W_{l,mn} - \frac{1}{2} B_{W_{l,mn}^i}(t) W_{l,mn}^2, \quad \text{(S5)}$$

$$\triangle_{f_{l,mi} \rightarrow u_{l-1,ni}}(t) \approx A_{u_{l-1,ni}^m}(t) u_{l-1,ni} - \frac{1}{2} B_{u_{l-1,ni}^m}(t) u_{l-1,ni}^2, \quad \text{(S6)}$$

where we define:

$$A_{b_{l,m}^i}(t) = \mu_{s_{l,mi}}(t) + v_{s_{l,mi}}(t) \mu_{b_{l,m}}(t),$$

$$B_{b_{l,m}^i}(t) = v_{s_{l,mi}}(t),$$

$$\begin{aligned} A_{W_{l,mn}^i}(t) = & \mu_{s_{l,mi}}(t) \mu_{u_{l-1,ni} \rightarrow f_{l,mi}}(t) \\ & + v_{s_{l,mi}}(t) \mu_{u_{l-1,ni}}^2(t) \mu_{W_{l,mn}}(t), \end{aligned}$$

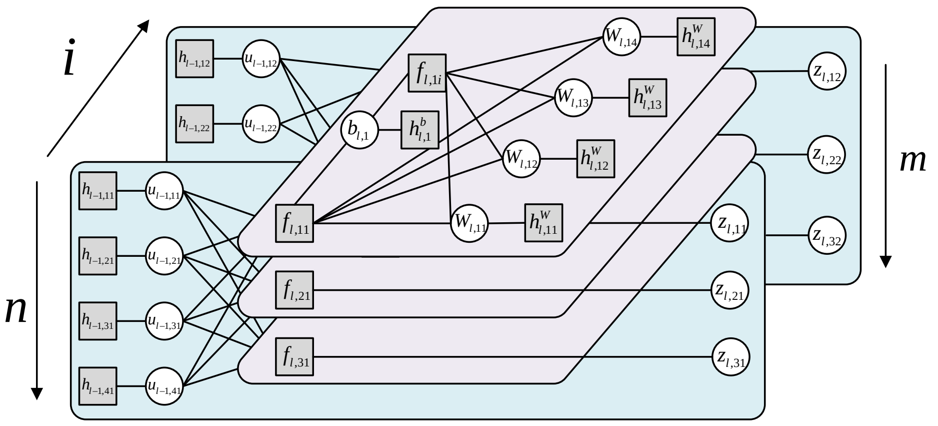


Fig. S1. Detailed structure of the $l$-th layer in $\mathcal{G}_{r_k}$, where we set $N_l = 3, N_{l-1} = 4, \mathcal{I}_{r_k} = \{1, 2\}$.

| | | | | | | | |
|---|---|---|---|---|---|---|---|
| $\mu_{b_{l,m}}$ | $O\left(\frac{1}{\sqrt{N}}\right)$ | $\mu_{b_{l,m}\to f_{l,mi}}$ | $O\left(\frac{1}{\sqrt{N}}\right)$ | $\mu_{b_{l,m}\to h^b_{l,m}}$ | $O\left(\frac{1}{\sqrt{N}}\right)$ | $\mu_{b_{l,m}\to f_{l,mi}} - \mu_{b_{l,m}}$ | $O\left(\frac{1}{N}\right)$ |
| $v_{b_{l,m}}$ | $O\left(\frac{1}{N}\right)$ | $v_{b_{l,m}\to f_{l,mi}}$ | $O\left(\frac{1}{N}\right)$ | $v_{b_{l,m}\to h^b_{l,m}}$ | $O\left(\frac{1}{N}\right)$ | $v_{b_{l,m}\to f_{l,mi}} - v_{b_{l,m}}$ | $O\left(\frac{1}{N^{3/2}}\right)$ |
| $\mu_{W_{l,mn}}$ | $O\left(\frac{1}{\sqrt{N}}\right)$ | $\mu_{W_{l,mn}\to f_{l,mi}}$ | $O\left(\frac{1}{\sqrt{N}}\right)$ | $\mu_{W_{l,mn}\to h^W_{l,mn}}$ | $O\left(\frac{1}{\sqrt{N}}\right)$ | $\mu_{W_{l,mn}\to f_{l,mi}} - \mu_{W_{l,mn}}$ | $O\left(\frac{1}{N}\right)$ |
| $v_{W_{l,mn}}$ | $O\left(\frac{1}{N}\right)$ | $v_{W_{l,mn}\to f_{l,mi}}$ | $O\left(\frac{1}{N}\right)$ | $v_{W_{l,mn}\to h^W_{l,mn}}$ | $O\left(\frac{1}{N}\right)$ | $v_{W_{l,mn}\to f_{l,mi}} - v_{W_{l,mn}}$ | $O\left(\frac{1}{N^{3/2}}\right)$ |
| $\mu_{u_{l-1,ni}}$ | $O(1)$ | $\mu_{u_{l-1,ni}\to f_{l,mi}}$ | $O(1)$ | $\mu_{u_{l-1,ni}\to h_{l-1,ni}}$ | $O(1)$ | $\mu_{u_{l-1,ni}\to f_{l,mi}} - \mu_{u_{l-1,ni}}$ | $O\left(\frac{1}{\sqrt{N}}\right)$ |
| $v_{u_{l-1,ni}}$ | $O(1)$ | $v_{u_{l-1,ni}\to f_{l,mi}}$ | $O(1)$ | $\mu_{u_{l-1,ni}\to h_{l-1,ni}}$ | $O(1)$ | $v_{u_{l-1,ni}\to f_{l,mi}} - v_{u_{l-1,ni}}$ | $O\left(\frac{1}{\sqrt{N}}\right)$ |
| $\mu_{z_{l,mi}}$ | $O(1)$ | $\mu_{f_{l,mi}\to z_{l,mi}}$ | $O(1)$ | $v_{s_{l,mi}}$ | $O(1)$ | | |
| $v_{z_{l,mi}}$ | $O(1)$ | $v_{f_{l,mi}\to z_{l,mi}}$ | $O(1)$ | $\mu_{s_{l,mi}}$ | $O(1)$ | | |

TABLE SI
VARIABLE SCALINGS IN THE LARGE SYSTEM LIMIT

$$B_{W^i_{l,mn}}(t) = v_{s_{l,mi}}(t)\,\mu^2_{u_{l-1,ni}}(t) - v_{u_{l-1,ni}}(t)\left(\mu^2_{s_{l,mi}}(t) - v_{s_{l,mi}}(t)\right),$$

$$A_{u^m_{l-1,ni}}(t) = \mu_{s_{l,mi}}(t)\,\mu_{W_{l,mn}\to f_{l,mi}}(t) + v_{s_{l,mi}}(t)\,\mu^2_{W_{l,mn}}(t)\,\mu_{u_{l-1,ni}}(t),$$

$$B_{u^m_{l-1,ni}}(t) = v_{s_{l,mi}}(t)\,\mu^2_{W_{l,mn}}(t) - v_{W_{l,mn}}(t)\left(\mu^2_{s_{l,mi}}(t) - v_{s_{l,mi}}(t)\right),$$

and

$$\mu_{s_{l,mi}}(t) = \frac{\partial \triangle_{f_{l,mi}\to x}(t)}{\partial \mu_{z_{l,mi}|x}}\Big|_{\mu_x(t)} = \frac{\mu_{z_{l,mi}}(t) - \mu_{f_{l,mi}\to z_{l,mi}}(t)}{v_{f_{l,mi}\to z_{l,mi}}(t)},$$

$$v_{s_{l,mi}}(t) = -\frac{\partial^2 \triangle_{f_{l,mi}\to x}(t)}{\partial \mu^2_{z_{l,mi}|x}}\Big|_{\mu_x(t)} = \frac{1}{v_{f_{l,mi}\to z_{l,mi}}(t)}\left(1 - \frac{v_{z_{l,mi}}(t)}{v_{f_{l,mi}\to z_{l,mi}}(t)}\right).$$

### *B. Approximated Variable-to-Factor Messages*

Here we approximate $\mu_{u_{l-1,ni}\to f_{l,mi}}(t+1), \mu_{W_{l,mn}\to f_{l,mi}}(t+1)$ and $\mu_{b_{l,m}\to f_{l,mi}}(t+1)$ based on Taylor series expansion. Firstly, we compute $\triangle_{u_{l-1,ni}\to f_{l,mi}}(t+1)$ based on sum product rule:

$$\triangle_{u_{l-1,ni}\to f_{l,mi}}(t+1) = \triangle_{h_{l-1,ni}\to u_{l-1,ni}} + \sum_{m'\neq m} \triangle_{f_{l,m'i}\to u_{l-1,ni}}(t).$$

Plugging in (S6), $\exp\left(\sum_{m'\neq m} \triangle_{f_{l,m'i}\to u_{l-1,ni}}(t)\right)$ is approximated as Gaussian with expectation and variance denoted by $\mu_{mni}(t)$ and $v_{mni}(t)$, respectively:

$$\begin{aligned}\mu_{mni}(t) &= \frac{\sum_{m'\neq m} A_{u^{m'}_{l-1,ni}}(t)}{\sum_{m'\neq m} B_{u^{m'}_{l-1,ni}}(t)} \\ &= \frac{\sum_{m=1}^{N_l} A_{u^m_{l-1,ni}}(t)}{\sum_{m=1}^{N_l} B_{u^m_{l-1,ni}}(t)} - \frac{\mu_{W_{l,mn}}(t)\,\mu_{s_{l,mi}}(t)}{\sum_{m=1}^{N_l} B_{u^m_{l-1,ni}}(t)} \\ &\quad + O\left(\frac{1}{N}\right) \\ &= \mu_{u_{l-1,ni}\to h_{l-1,ni}}(t) \\ &\quad - \mu_{W_{l,mn}}(t)\,\mu_{s_{l,mi}}(t)\,v_{u_{l-1,ni}\to h_{l-1,ni}}(t) \\ &\quad + O\left(\frac{1}{N}\right),\end{aligned}$$

$$v_{mni}(t) = \frac{1}{\sum_{m' \neq m} B_{u^{m'}_{l-1,ni}}(t)} = \frac{1}{\sum_{m=1}^{N_l} B_{u^{m}_{l-1,ni}}(t)} + O\left(\frac{1}{N}\right) = v_{u_{l-1,ni} \to h_{l-1,ni}}(t) + O\left(\frac{1}{N}\right).$$

By applying Taylor series expansion and omit $O\left(\frac{1}{N}\right)$ terms, we obtain the approximated $\mu_{u_{l-1,ni} \to f_{l,mi}}(t+1)$:

$$\begin{aligned}\mu_{u_{l-1,ni} \to f_{l,mi}}(t+1) &\approx \int_{u_{l-1,ni}} u_{l-1,ni} \exp\left(\triangle_{h_{l-1,ni} \to u_{l-1,ni}}\right) \\ &\times N\left(u_{l-1,ni}; \mu_{mni}(t), v_{mni}(t)\right) \\ &\approx \mu_{u_{l-1,ni}}(t+1) \\ &- \mu_{W_{l,mn}}(t)\, \mu_{s_{l,mi}}(t)\, v_{u_{l-1,ni}}(t+1).\end{aligned} \tag{S7}$$

Similarly, we obtain:

$$\begin{aligned}\mu_{W_{l,mn} \to f_{l,mi}}(t+1) &\approx \mu_{W_{l,mn}}(t+1) \\ &- \mu_{u_{l-1,ni}}(t)\, \mu_{s_{l,mi}}(t)\, v_{u_{l-1,ni}}(t+1),\end{aligned} \tag{S8}$$

$$\mu_{b_{l,m} \to f_{l,mi}}(t+1) \approx \mu_{b_{l,m}}(t+1). \tag{S9}$$

### C. Closing the Loop

In the following, we plug in the approximated results of messages on edge to give the updating rules for forward messages and backward messages. Firstly, we consider forward message $\triangle_{f_{l,mi} \to z_{l,mi}}(t)$. Plugging (S7), (S8) and (S9) in (S2) and (S3), we obtain:

$$\mu_{f_{l,mi} \to z_{l,mi}}(t) \approx \mu_{p_{l,mi}}(t) - \mu_{s_{l,mi}}(t-1)\, v_{p_{l,mi}}(t),$$

$$v_{f_{l,mi} \to z_{l,mi}}(t) \approx v_{p_{l,mi}}(t) + \sum_{n=1}^{N_{l-1}} v_{W_{l,mn}}(t)\, v_{u_{l-1,ni}}(t) + v_{b_{l,m}}(t),$$

where we define

$$\mu_{p_{l,mi}}(t) = \sum_{n=1}^{N_{l-1}} \mu_{W_{l,mn}}(t)\, \mu_{u_{l-1,ni}}(t) + \mu_{b_{l,m}}(t),$$

$$v_{p_{l,mi}}(t) = \sum_{n=1}^{N_{l-1}} \mu^2_{W_{l,mn}}(t)\, v_{u_{l-1,ni}}(t) + \sum_{n=1}^{N_{l-1}} v_{W_{l,mn}}(t)\, \mu^2_{u_{l-1,ni}}(t).$$

Next, we update aggregated backward messages $\triangle_{b_{l,m} \to h^b_{l,m}}(t), \triangle_{W_{l,mn} \to h^W_{l,mn}}(t), \triangle_{u_{l-1,ni} \to h_{l-1,ni}}(t)$ based on sum product rule:

$$\triangle_{b_{l,m} \to h^b_{l,m}}(t) = \sum_{i \in \mathcal{I}_{r_k}} \triangle_{f_{l,mi} \to b_{l,m}}(t),$$

$$\triangle_{W_{l,mn} \to h^W_{l,mn}}(t) = \sum_{i \in \mathcal{I}_{r_k}} \triangle_{f_{l,mi} \to W_{l,mn}}(t),$$

$$\triangle_{u_{l-1,ni} \to h_{l-1,ni}}(t) = \sum_{m=1}^{N_l} \triangle_{f_{l,mi} \to u_{l-1,ni}}(t).$$

Plugging in (S4), (S5),(S6), we obtain:

$$v_{b_{l,m} \to h^b_{l,m}}(t) = \left(\sum_{i \in \mathcal{I}_{r_k}} v_{s_{l,mi}}(t)\right)^{-1},$$

$$\mu_{b_{l,m} \to h^b_{l,m}}(t) = \mu_{b_{l,m}}(t) + \frac{\sum_{i \in \mathcal{I}_{r_k}} \mu_{s_{l,mi}}(t)}{\sum_{i \in \mathcal{I}_{r_k}} v_{s_{l,mi}}(t)},$$

$$v_{W_{l,mn} \to h^W_{l,mn}}(t) \approx \left(v_{s_{l,mi}}(t)\, \mu^2_{u_{l-1,ni}}(t)\right)^{-1},$$

$$\mu_{W_{l,mn} \to h^W_{l,mn}}(t) = \mu_{W_{l,mn}}(t)\left(1 - G_{W_{l,mn}}(t)\right) + v_{W_{l,mn} \to h^W_{l,mn}}(t) \sum_{i \in \mathcal{I}_{r_k}} \mu_{u_{l-1,ni}}(t)\, \mu_{s_{l,mi}}(t),$$

$$v_{u_{l-1,ni} \to h_{l-1,ni}}(t) \approx \left(v_{s_{l,mi}}(t)\, \mu^2_{W_{l,mn}}(t)\right)^{-1},$$

$$\mu_{u_{l-1,ni} \to h_{l-1,ni}}(t) = \mu_{u_{l-1,ni}}(t)\left(1 - G_{u_{l-1,ni}}(t)\right) + v_{u_{l-1,ni} \to h_{l-1,ni}}(t) \sum_{m=1}^{N_l} \mu_{W_{l,mn}}(t)\, \mu_{s_{l,mi}}(t),$$

where $\mu_{b_{l,m} \to f_{l,mi}}(t+1), \mu_{W_{l,mn} \to f_{l,mi}}(t+1), \mu_{u_{l-1,ni} \to f_{l,mi}}(t+1)$ are replaced with (S7),(S8),(S9), and we define:

$$G_{W_{l,mn}}(t) = v_{W_{l,mn} \to h^W_{l,mn}}(t) \sum_{i \in \mathcal{I}_{r_k}} v_{u_{l-1,ni}}(t)\, v_{s_{l,mi}}(t),$$

$$G_{u_{l-1,ni}}(t) = v_{u_{l-1,ni} \to h_{l-1,ni}}(t) \sum_{m=1}^{N_l} v_{W_{l,mn}}(t)\, v_{s_{l,mi}}(t).$$

### D. Algorithm Summary

The derivation above is summarized in Algorithm 1 and 2, where we separate forward and backward message passing and omit iteration-$t$. Because in DAMP algorithm, each layer does not update messages in turn independently, and the overall schedule during iterations is given in the main text.

**Algorithm 1** Approximated forward message passing within layer $l$

Update $\forall m: \mu_{b_{l,m}}, v_{b_{l,m}}$ with $\triangle_{b_{l,m}} = \triangle_{b_{l,m}\to h^b_{l,m}} + \triangle_{h^b_{l,m}\to b_{l,m}}$.

Update $\forall m,n: \mu_{W_{l,mn}}, v_{W_{l,mn}}$ with $\triangle_{W_{l,mn}} = \triangle_{W_{l,mn}\to h^W_{l,mn}} + \triangle_{h^W_{l,mn}\to W_{l,mn}}$.

Update $\forall n,i: \mu_{u_{l-1,ni}}, v_{u_{l-1,ni}}$ with $\triangle_{u_{l-1,ni}} = \triangle_{u_{l-1,ni}\to h_{l-1,ni}} + \triangle_{h_{l-1,ni}\to u_{l-1,ni}}$.

$\forall m,i: \mu_{p_{l,mi}} = \sum_{n=1}^{N_{l-1}} \mu_{W_{l,mn}}\mu_{u_{l-1,ni}} + \mu_{b_{l,m}}$

$\forall m,i: v_{p_{l,mi}} = \sum_{n=1}^{N_{l-1}} \left(\mu^2_{W_{l,mn}} v_{u_{l-1,ni}} + v_{W_{l,mn}}\mu^2_{u_{l-1,ni}}\right)$

$\forall m,i: \mu_{f_{l,mi}\to z_{l,mi}} = \mu_{p_{l,mi}} - \mu_{s_{l,mi}} v_{p_{l,mi}}$

$\forall m,i: v_{f_{l,mi}\to z_{l,mi}}$
$= v_{p_{l,mi}} + \sum_{n=1}^{N_{l-1}} v_{W_{l,mn}} v_{u_{l-1,ni}} + v_{b_{l,m}}$

Output $\forall m,i: \triangle_{f_{l,mi}\to z_{l,mi}}$
$= \log N\left(z_{l,mi}; \mu_{f_{l,mi}\to z_{l,mi}}, v_{f_{l,mi}\to z_{l,mi}}\right)$

**Algorithm 2** Approximated backward message passing within layer $l$

Update $\forall m,i: \mu_{z_{l,mi}}, v_{z_{l,mi}}$ with $\triangle_{z_{l,mi}} = \triangle_{f_{l,mi}\to z_{l,mi}} + \triangle_{z_{l,mi}\to f_{l,mi}}$.

$\forall m,i: v_{s_{l,mi}} = \left(1 - v_{z_{l,mi}}/v_{f_{l,mi}\to z_{l,mi}}\right)/v_{f_{l,mi}\to z_{l,mi}}$

$\forall m,i: \mu_{s_{l,mi}} = \left(\mu_{z_{l,mi}} - \mu_{f_{l,mi}\to z_{l,mi}}\right)/v_{f_{l,mi}\to z_{l,mi}}$

$\forall m: v_{b_{l,m}\to h^b_{l,m}} = \left(\sum_{i\in\mathcal{I}_{r_k}} v_{s_{l,mi}}\right)^{-1}$

$\forall m: \mu_{b_{l,m}\to h^b_{l,m}} = \mu_{b_{l,m}} + v_{b_{l,m}\to h^b_{l,m}} \sum_{i\in\mathcal{I}_{r_k}} \mu_{s_{l,mi}}$

Update $\forall m: \triangle_{b_{l,m}\to h^b_{l,m}}$
$= \log N\left(b_{l,m}; \mu_{b_{l,m}\to h^b_{l,m}}, v_{b_{l,m}\to h^b_{l,m}}\right)$.

$\forall m,n: v_{W_{l,mn}\to h^W_{l,mn}} = \left(\sum_{i\in\mathcal{I}_{r_k}} \mu^2_{u_{l-1,ni}} v_{s_{l,mi}}\right)^{-1}$

$\forall m,n: G_{W_{l,mn}} = v_{W_{l,mn}\to h^W_{l,mn}} \sum_{i\in\mathcal{I}_{r_k}} v_{u_{l-1,ni}} v_{s_{l,mi}}$.

$\forall m,n: \mu_{W_{l,mn}\to h^W_{l,mn}} = \mu_{W_{l,mn}}\left(1 - G_{W_{l,mn}}\right)$
$+ v_{W_{l,mn}\to h^W_{l,mn}} \sum_{i\in\mathcal{I}_{r_k}} \mu_{u_{l-1,ni}}\mu_{s_{l,mi}}$.

Update $\forall m,n: \triangle_{W_{l,mn}\to h^W_{l,mn}}$
$= \log N\left(W_{l,mn}; \mu_{W_{l,mn}\to h^W_{l,mn}}, v_{W_{l,mn}\to h^W_{l,mn}}\right)$.

$\forall n,i: v_{u_{l-1,ni}\to h_{l-1,ni}} = \left(\sum_{m=1}^{N_l} \mu^2_{W_{l,mn}} v_{s_{l,mi}}\right)^{-1}$

$\forall n,i: G_{u_{l-1,ni}} = v_{u_{l-1,ni}\to h_{l-1,ni}} \sum_{m=1}^{N_l} v_{W_{l,mn}} v_{s_{l,mi}}$.

$\forall n,i: \mu_{u_{l-1,ni}\to h_{l-1,ni}} = \mu_{u_{l-1,ni}}\left(1 - G_{u_{l-1,ni}}\right)$
$+ v_{u_{l-1,ni}\to h_{l-1,ni}} \sum_{m=1}^{N_l} \mu_{W_{l,mn}}\mu_{s_{l,mi}}$.

Output $\forall n,i: \triangle_{u_{l-1,ni}\to h_{l-1,ni}}$
$= \log N\left(u_{l-1,ni}; \mu_{u_{l-1,ni}\to h_{l-1,ni}}, v_{u_{l-1,ni}\to h_{l-1,ni}}\right)$.

## S-II. Expectation and Variance for Messages Related to Nonlinear Steps

In the main text, we derive the messages related to nonlinear steps. However, the related expectations and variances instead of messages are used during iterations in Algorithm 1 and 2. Therefore, in the following we give the specific expectations and variances w.r.t. messages related to nonlinear steps, where we adopt the notations defined in the main text.

### A. ReLU Activation Function

Based on derivation in the main text, both $\exp\left(\triangle_u\right)$ and $\exp\left(\triangle_z\right)$ are sum of truncated normal distribution. The related expectation and variance are given as follows:

$$\mu_u = \frac{H\left(-\mu_0, v_0\right)\mu_0 + v_0}{H\left(\mu_{f\to z}, v_{f\to z}\right) + H\left(-\mu_0, v_0\right)},$$

$$v_u = \frac{H\left(-\mu_0, v_0\right)\left(\mu_0^2 + v_0\right) + \mu_0 v_0}{H\left(\mu_{f\to z}, v_{f\to z}\right) + H\left(-\mu_0, v_0\right)} - \mu_u^2,$$

$$\mu_z = \frac{\mu_{f\to z} H\left(\mu_{f\to z}, v_{f\to z}\right) + \mu_0 H\left(-\mu_0, v_0\right) + v_0 - v_{f\to z}}{H\left(\mu_{f\to z}, v_{f\to z}\right) + H\left(-\mu_0, v_0\right)},$$

$$v_z = \frac{\left(\mu^2_{f\to z} + v_{f\to z}\right) H\left(\mu_{f\to z}, v_{f\to z}\right) + \left(\mu_0^2 + v_0\right) H\left(-\mu_0, v_0\right)}{H\left(\mu_{f\to z}, v_{f\to z}\right) + H\left(-\mu_0, v_0\right)} + \frac{\mu_0 v_0 - \mu_{f\to z} v_{f\to z}}{H\left(\mu_{f\to z}, v_{f\to z}\right) + H\left(-\mu_0, v_0\right)} - \mu_z^2,$$

where for convenience, we define:

$$H\left(\mu, v\right) = \frac{Q\left(\frac{\mu}{\sqrt{v}}\right)}{N\left(\mu, v\right)},$$

$$v_0 = \frac{v_{f\to z} v_{u\to h}}{v_{f\to z} + v_{u\to h}}, \mu_0 = \frac{\mu_{u\to h} v_{f\to z} + \mu_{f\to z} v_{u\to h}}{v_{f\to z} + v_{u\to h}}.$$

### B. Probit-product Likelihood Function

In the main text, we approximate the skew normal distributions $\exp\left(\triangle_{z_{y,m}}\right)$ and $\exp\left(\triangle_{z_m}\right)$ for $m \neq y$ as Gaussian based on moment matching. Here we directly give the expectations and variances:

$$\mu_{z_{y,m}} = \mu_{f_y\to z_y} + v_{f_y\to z_y} H_{y,m},$$

$$v_{z_{y,m}} = v_{f_y\to z_y} + v^2_{f_m\to z_m} \frac{\mu_{f_m\to z_m} - \mu_{f_y\to z_y}}{v_{f_m\to z_m} + v_{f_y\to z_y} + v} H_{y,m} - v^2_{f_y\to z_y} H^2_{y,m},$$

$$\mu_{z_m} = \mu_{f_m\to z_m} - v_{f_m\to z_m} H_m,$$

$$v_{z_m} = v_{f_m\to z_m} + v^2_{f_m\to z_m} \frac{\mu_{f_m\to z_m} - \mu_{z_y\to h_m}}{v_{f_m\to z_m} + v_{z_y\to h_m} + v} H_m - v^2_{f_m\to z_m} H^2_m,$$

where we define:

$$H_{y,m} = H\left(\mu_{f_m\to z_m} - \mu_{f_y\to z_y}, v_{f_m\to z_m} + v_{f_y\to z_y} + v\right),$$

$$H_m = H\left(\mu_{f_m\to z_m} - \mu_{z_y\to h_m}, v_{f_m\to z_m} + v_{z_y\to h_m} + v\right).$$

## S-III. Specific expression for global posterior distribution $p(\boldsymbol{\theta}|\boldsymbol{D})$

In the proposed Bayesian federated learning framework, we approximate the global posterior distribution $p(\boldsymbol{\theta}|\boldsymbol{D})$ as the weighted geometric average of local posterior distributions $p\left(\boldsymbol{\theta}|\boldsymbol{D}^k\right), k=1,\ldots,K$ [S2]:

$$p(\boldsymbol{\theta}|\boldsymbol{D}) \approx \prod_{k=1}^{K}\left(p\left(\boldsymbol{\theta}|\boldsymbol{D}^k\right)\right)^{\frac{I_k}{I}}, \tag{S10}$$

where $p\left(\boldsymbol{\theta}|\boldsymbol{D}^k\right)$ is approximated as the product of marginal posterior distributions (which has been widely used in the literature since the marginal posterior distributions can be efficiently computed using the factor graph and message passing approach):

$$p\left(\boldsymbol{\theta}|\boldsymbol{D}^k\right) \approx \prod_{m=1}^{Q_b} p\left(b_m|\boldsymbol{D}^k\right)\prod_{i=1}^{Q_W} p\left(\boldsymbol{W}_{n\in\mathcal{N}_i}|\boldsymbol{D}^k\right),$$

where the marginal posterior distributions are group Bernoulli-Gaussian denoted as follows:

$$p\left(b_m|\boldsymbol{D}^k\right) = \rho_{b_m,k} N\left(b_m;\mu_{b_m,k},v_{b_m,k}\right) + \left(1-\rho_{b_m,k}\right)\delta\left(b_m\right),$$

$$\begin{aligned} p\left(\boldsymbol{W}_{n\in\mathcal{N}_i}|\boldsymbol{D}^k\right) = {} & \rho_{W_i,k}\prod_{n\in\mathcal{N}_i} N\left(W_{i,n};\mu_{W_{i,n},k},v_{W_{i,n},k}\right) \\ & + \left(1-\rho_{W_i,k}\right)\prod_{n\in\mathcal{N}_i}\delta\left(W_{i,n}\right). \end{aligned}$$

For convenience, we denote the local posterior parameters $\boldsymbol{\varphi}^k$ as a set consisting of $\rho_{b_m,k},\mu_{b_m,k},v_{b_m,k}$ for $m=1,\cdots,Q_b$ and $\rho_{W_i,k},\mu_{W_{i,n},k},v_{W_{i,n},k}$ for $i=1,\cdots,Q_W, n\in\mathcal{N}_i$, which are sent to the central server in uplink communication. Notice that when the local posterior distributions are products of group Bernoulli-Gaussian, it is difficult to derive the exact expression for the global posterior distribution based on (S10). Thus, we approximate the global posterior distribution as product of group Bernoulli-Gaussian:

$$q(\boldsymbol{\theta}) = \prod_{m=1}^{Q_b} q_{b_m}\left(b_m\right)\prod_{i=1}^{Q_W} q_{W_i}\left(\boldsymbol{W}_{n\in\mathcal{N}_i}\right),$$

$$q_{b_m}\left(b_m\right) = \rho_{b_m} N\left(b_m;\mu_{b_m},v_{b_m}\right) + \left(1-\rho_{b_m}\right)\delta\left(b_m\right),$$

$$\begin{aligned} q_{W_i}\left(\boldsymbol{W}_{n\in\mathcal{N}_i}\right) = {} & \rho_{W_i}\prod_{n\in\mathcal{N}_i} N\left(W_{i,n};\mu_{W_{i,n}},v_{W_{i,n}}\right) \\ & + \left(1-\rho_{W_i}\right)\prod_{n\in\mathcal{N}_i}\delta\left(W_{i,n}\right), \end{aligned}$$

where the parameters are chosen by minimizing the Kullback-Leibler divergence $D_{KL}\left(p(\boldsymbol{\theta}|\boldsymbol{D})\,||\,q(\boldsymbol{\theta})\right)$, and $p(\boldsymbol{\theta}|\boldsymbol{D})$ is given in (S10). The detailed derivation is omitted, and we directly present the updating rules:

$$\mu_{b_m} = \frac{\sum_{k=1}^{K}\frac{I_k\mu_{b_m,k}}{Iv_{b_m,k}}}{\sum_{k=1}^{K}\frac{I_k}{Iv_{b_m,k}}}, v_{b_m} = \frac{1}{\sum_{k=1}^{K}\frac{I_k}{Iv_{b_m,k}}}, \tag{S11}$$

$$\rho_{b_m} = \frac{1}{1+\frac{1}{C_{b_m}}\prod_{k=1}^{K}\left(\frac{1-\rho_{b_m,k}}{\rho_{b_m,k}}\right)^{\frac{I_k}{I}}}, \tag{S12}$$

$$\mu_{W_{i,n}} = \frac{1}{\sum_{k=1}^{K}\frac{I_k}{Iv_{W_{i,n},k}}}, v_{W_{i,n}} = \frac{\sum_{k=1}^{K}\frac{I_k\mu_{W_{i,n},k}}{Iv_{W_{i,n},k}}}{\sum_{k=1}^{K}\frac{I_k}{Iv_{W_{i,n},k}}}, \tag{S13}$$

$$\rho_{W_i} = \frac{1}{1+\frac{1}{C_{W_i}}\prod_{k=1}^{K}\left(\frac{1-\rho_{W_i,k}}{\rho_{W_i,k}}\right)^{\frac{I_k}{I}}}, \tag{S14}$$

where

$$C_{b_m} = \frac{\prod_{k=1}^{K}\left(N\left(\mu_{b_m,k},v_{b_m,k}\right)\right)^{\frac{I_k}{I}}}{N\left(\mu_{b_m},v_{b_m}\right)},$$

$$C_{W_i} = \prod_{n\in\mathcal{N}_i}\left(\frac{\prod_{k=1}^{K}\left(N\left(\mu_{W_{i,n},k},v_{W_{i,n},k}\right)\right)^{\frac{I_k}{I}}}{N\left(\mu_{W_{i,n}},v_{W_{i,n}}\right)}\right).$$

As mentioned in the main text, parameters in $\boldsymbol{\psi}$ can be updated as (S11)-(S14) correspondingly.

## References


[S1] J. T. Parker, P. Schniter, and V. Cevher, "Bilinear generalized approximate message passing—part i: Derivation," *IEEE Transactions on Signal Processing*, vol. 62, no. 22, pp. 5839–5853, Nov. 2014.

[S2] L. Liu, X. Jiang, F. Zheng, H. Chen, G.-J. Qi, H. Huang, and L. Shao, "A bayesian federated learning framework with online laplace approximation," *IEEE Trans. Pattern Anal. Mach. Intell.*, vol. 46, no. 1, pp. 1–16, Jan. 2024.
